# Supplementary material for: Mapping of shadows cast on a protoplanetary disk by a close binary system
Source: arXiv:1811.10621 source file (2018-11-26)
Supplement: Supplementary file 1 [file supplementary_information.pdf]

# Mapping of shadows cast on a protoplanetary disc from a close binary system

## Supplementary Information

Supplementary Table 1: Astrophysical parameters of the V4046 Sgr system, namely binary period, inclination of the disc, distance of the system (in pc), locations of the inner and outer rings (in au), and flaring angles as calculated for the inner and outer disc rings. The corresponding errors are 1-sigma. References are given in the last Column.

| | | |
|---|---|---|
| **Binary Period** | **2.42129516±0.00003123** days | **This work** |
| Inclination of the disc | $33.5^{+0.7}_{-1.4}$ deg | Rosenfeld et al. (2012) |
| Distance | **78± 8 pc** | **This work** |
| Inner-ring radius | 13 au | This work and Rosenfeld et al. (2013) |
| Outer-ring radius | 29 au | This work and Rapson et al. (2015b) |
| $\alpha$ (inner) | **6.2±0.6** deg | **This work** |
| $\alpha$ (outer) | **8.5±1.0** deg | **This work** |

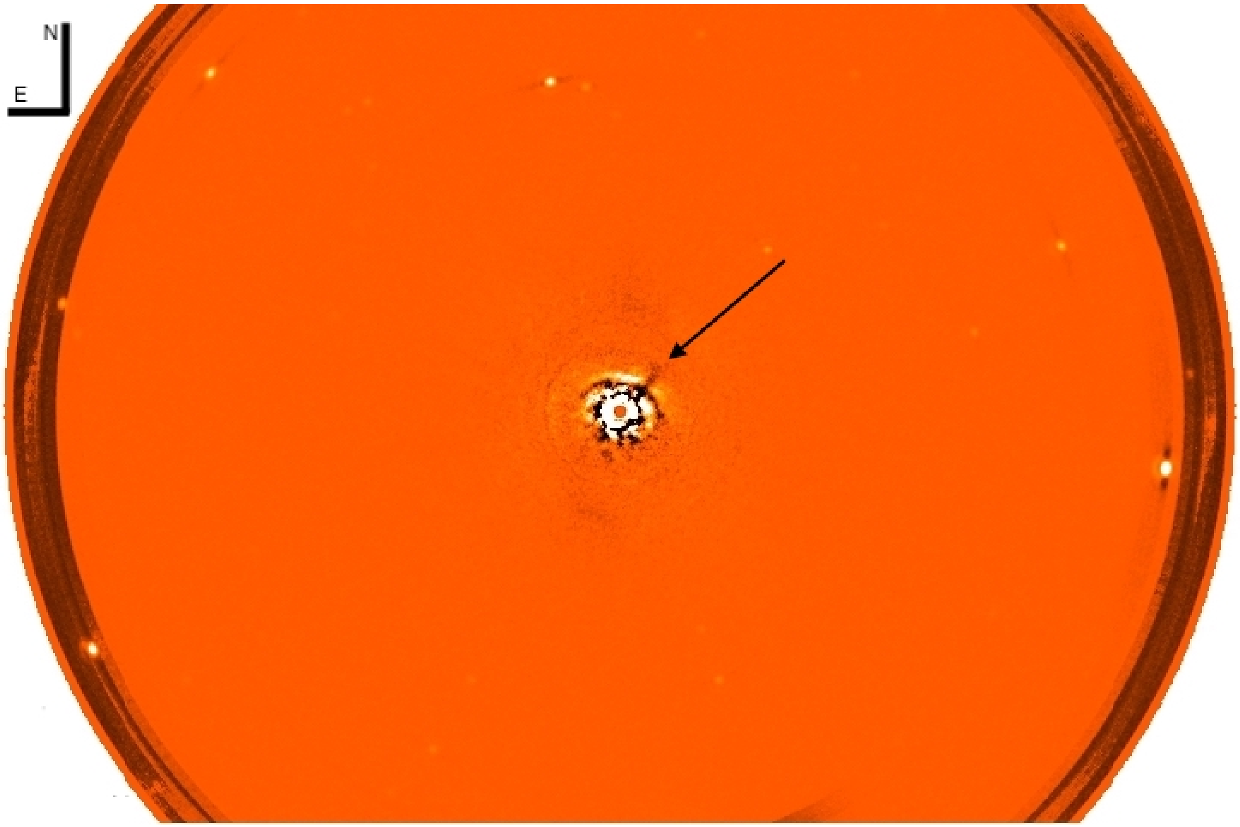


Supplementary Figure 1: Results of the TLOCI algorithm applied to IRDIS $K_1K_2$ observations for V4046 Sgr (observing epoch 2017). The field of view is 11" $\times$ 11" , with a pixel scale of 12.25 mas/pixel. The shadow location for the near side of the disc is clearly visible (black arrow). The sources located in the IRDIS field have been checked to be background objects.

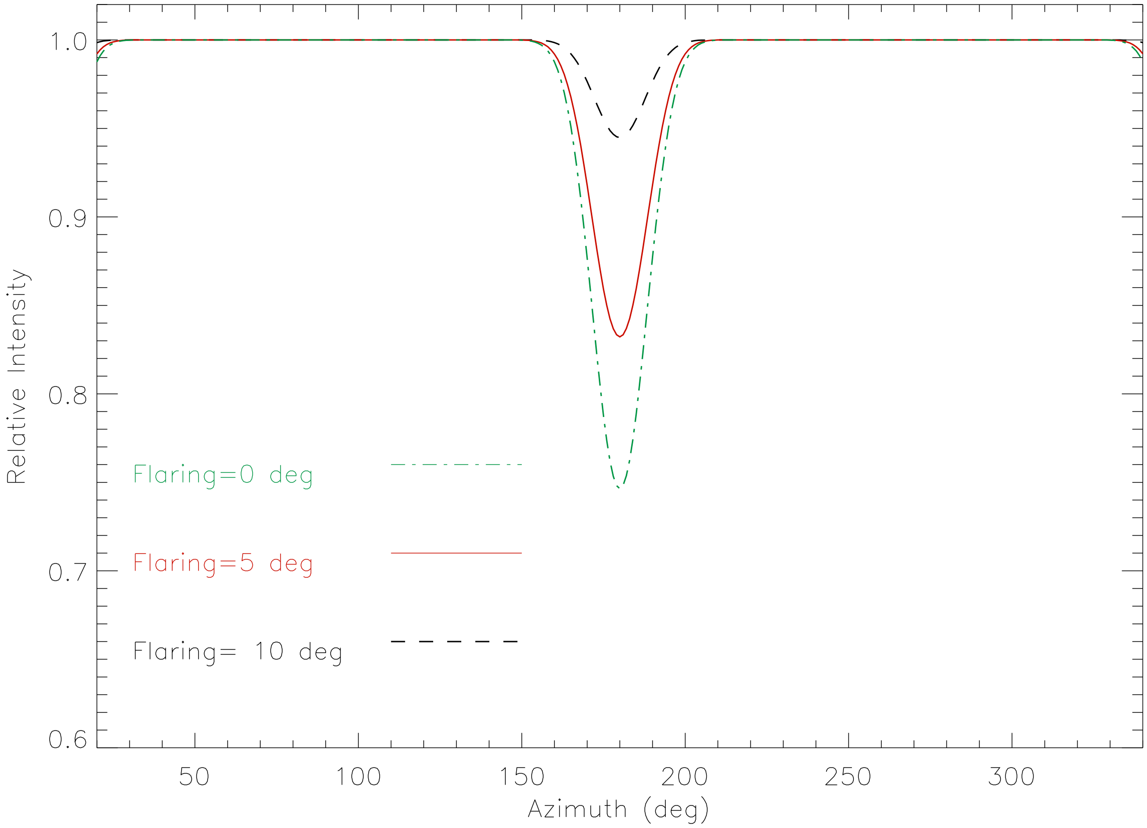


Supplementary Figure 2: Relative intensity of the shadow depth for different flaring angles of 0 (green, dot-dashed line), 5 (red solid line), and 10 (black dashed line) degrees.

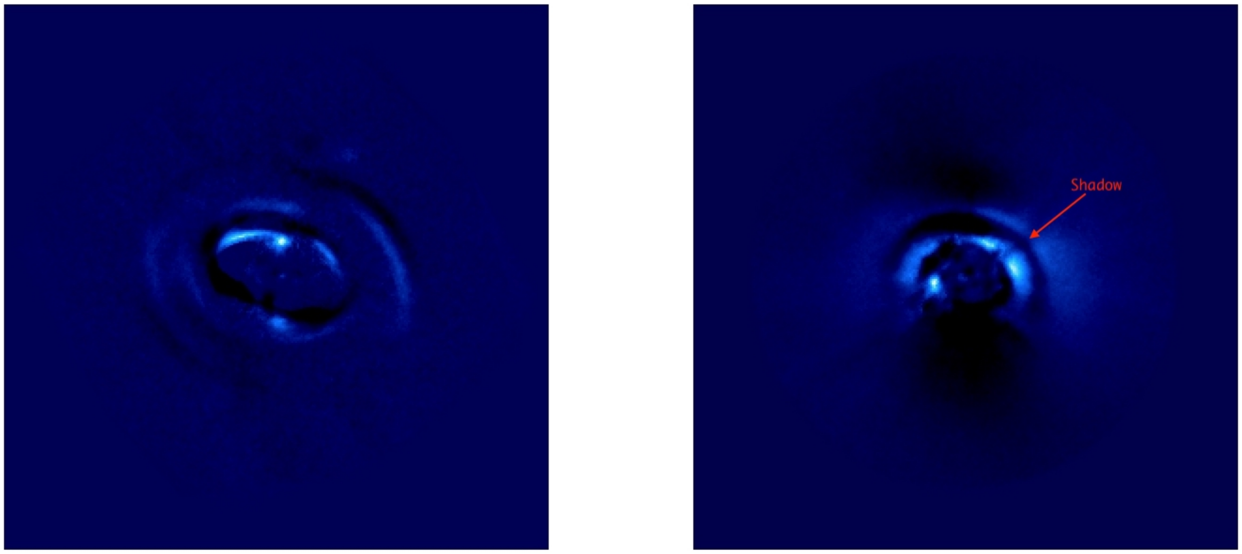


Supplementary Figure 3: Comparison between the ADI simulation (left-hand panel) and the IFS observations of V4046 Sgr (right-hand panel). Orientation and scale are as for Figure 1. ADI tends to create artefacts along the minor axis, which is not where the shadow is located in the real images.

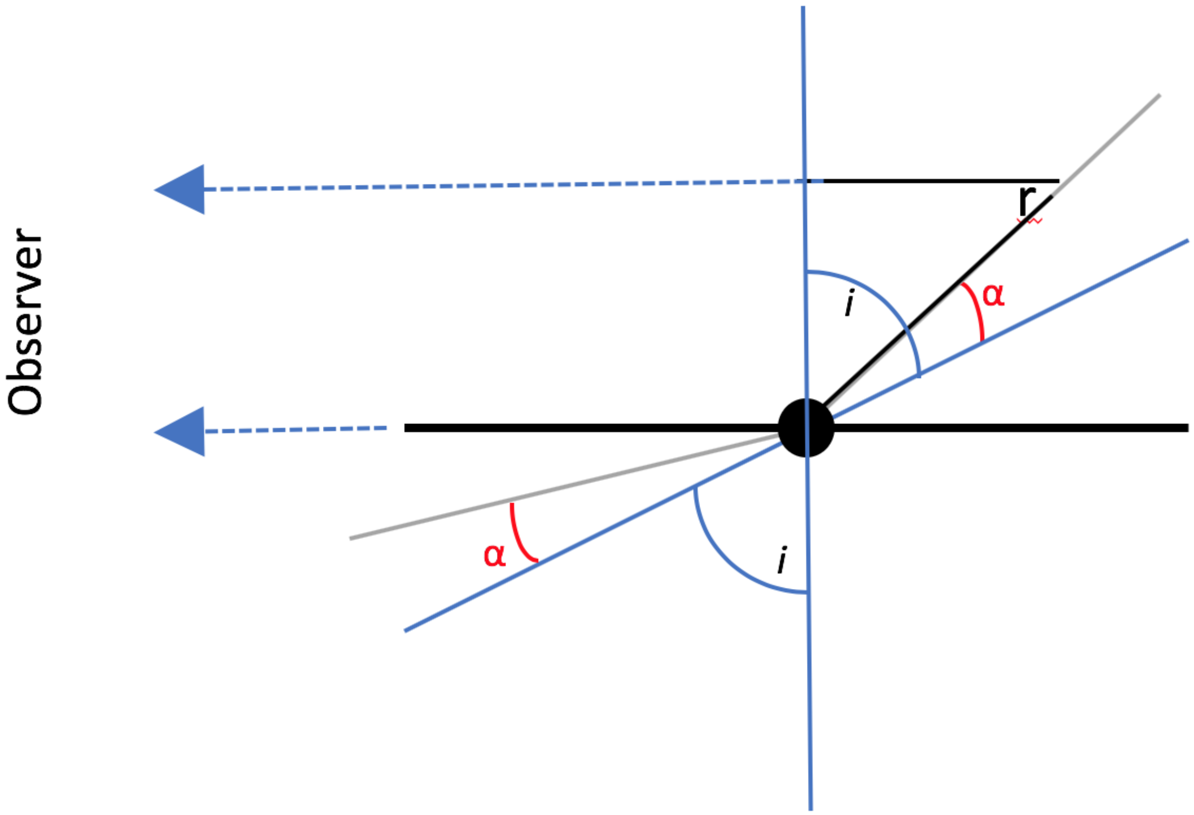


Supplementary Figure 4: Geometrical sketch of the system configuration. The flaring angle $\alpha$, the inclination angle of the disc (i), and the distance of the ring $r$ are marked.
